# Supplementary material for: A Plague of Magnetic Spots Among the Hot Stars of Globular Clusters
Source: arXiv:2006.02308 source file (2020-06-05)
Supplement: Supplementary file 1 [file Momany_SI_ASTROPH.pdf]

# Supplementary Information for

# A Plague of Magnetic Spots Among the Hot Stars of Globular Clusters

Y. Momany[1], S. Zaggia[1], M. Montalto[2], D. Jones[3,4], H.M.J. Boffin[5], S. Cassisi[6,7], C. Moni Bidin[8], M. Gullieuszik[1], I. Saviane[9], L. Monaco[10], E. Mason[11], L. Girardi[1], V. D'Orazi[1], G. Piotto[2], A.P. Milone[2], H. Lala[2], P.B. Stetson[12] & Y. Beletsky[13]

[1]*INAF - Osservatorio Astronomico di Padova, Vic. dell'Osservatorio 5, 35122 Padova, Italy*
[2]*Dipartimento di Fisica e Astronomia, Univ. di Padova, V. dell'Osservatorio 3, 35122 Padova, Italy*
[3]*Instituto de Astrofisica de Canarias, E-38205 La Laguna, Tenerife, Spain*
[4]*Departamento de Astrofisica, Universidad de La Laguna, E-38206 La Laguna, Tenerife, Spain*
[5]*European Southern Observatory, Karl Schwarzschild Strasse 2, D-85748 Garching, Germany*
[6]*INAF - Osservatorio Astronomico d'Abruzzo, Via M. Maggini, I-64100 Teramo, Italy*
[7]*INFN - Sezione di Pisa, Largo Pontecorvo 3, 56127 Pisa, Italy*
[8]*Instituto de Astronomía, Universidad Católica del Norte, Av. Angamos 0610, Antofagasta, Chile*
[9]*European Southern Observatory, Alonso de Cordova 3107, Santiago, Chile*
[10]*Departamento de Ciencias Fisicas, Universidad Andres Bello, Fernandez Concha 700, Las Condes, Santiago, Chile*
[11]*INAF - Osservatorio Astronomico di Trieste, Via G.B. Tiepolo, 11, I-34143, Trieste, Italy*
[12]*Herzberg Astronomy and Astrophysics, National Research Council, 5071 West Saanich Road, Victoria, BC V9E 2E7, Canada*
[13]*Las Campanas Observatory, Carnegie Institution of Washington, Colina el Pino, Casilla 601, La Serena, Chile*

## Supplementary Discussion

**The Stability of Magnetic Spots:** The parallelism we draw between the $\alpha^2$ CVn variability in magnetic $B_P$ stars and our EHB variables implies that the EHB variability should be stable on timescales of years. Supplementary Fig. 4 displays the six phased one-year light curves of vEHB-1/V16 in NGC6752 ($P \sim 19.5$ days) along with the integrated six-year curve and its corresponding best fitting model. Although the measurements originate from two different OmegaCAM data-sets, overall, there are no appreciable phase and amplitude differences among the six one-year light curves with respect to the integrated model. One therefore concludes that the observed EHB variability - attributed to magnetic spots - is stable on a timescale of years as is expected if belonging to the $\alpha^2$ CVn family.

The confirmed long-term stability of magnetic spots allows us to probe an important stellar property: rotation. A rotating stellar spot is an excellent probe of the *stellar* rotation, to the degree of being considered *superior*[1] to the spectroscopic $v\sin i$ measurements (which include assumptions on the rotation axis inclination). For example, a modelling of the $T_{eff} \sim 20,500\,\mathrm{K}$ vEHB-1 variable in NGC2808 implies a radius of $\sim 0.45\,\mathrm{R}_\odot$, which combined with a photometric period of $\sim 3.3$ days, translates into a stellar rotation velocity of $\sim 6.1$ km/s. This is in *perfect* agreement with conclusions of EHB $v\sin i$ studies (specifically in NGC2808[2]) being $\lesssim 10$ km/s. Repeating the same exercise, the $\sim 2-50$ days period distribution translates to a rotational velocity range between $\sim 0.4-10.0$ km/s. The $\sim 0.4$ km/s lower limit, lends support to earlier suggestions[2] that a small NGC2808 EHB population may display extremely low ($\lesssim 2$ km/s) rotational velocities. This overall consistency lends further support to the $\alpha^2$ CVn framework in explaining the EHB variability.

**Magnetism in Radiative Envelopes:** We emphasise that whereas the envisaged dynamo-generated magnetic fields actually *reach* the stellar surface[3], the trigger itself (i.e. HeIICZ) *remains*[4–6] *a sub-surface* layer (beneath a very-thin radiative layer) for the *entire* temperature range of our EHB variables. Indeed, atomic diffusion (in and around the EHB variables) is far from being suppressed by HeIICZ surface convection and, if anything, it gets weirder. In particular, we recall that the measured[7] surface Helium-abundances shows a smooth, increasing, trend between $\sim 15,000\,\mathrm{K}$ ($Y \sim 0.008$) and $\sim 20,000\,\mathrm{K}$ ($Y \sim 0.05$). However, for EHBs hotter than the M-jump, this trend is suddenly broken and replaced by a significant dispersion in surface Helium-abundances: varying anywhere between $0.001 \lesssim Y \lesssim 0.1$ on a star-to-star basis. Thus, the empirical Helium-abundance framework is still in perfect agreement with the EHBs' radiative envelopes showing diffusion effects and a general Helium-depletion. In this regard, one must bear in mind that an average EHB measured Helium-abundance of $Y \sim 0.05$ (still sign of "Helium-depletion") is still one order of magnitude *larger* than that theorised/expected assuming an equilibrium between the competing gravitational settling and radiative levitation processes. Weak stellar winds rendering less-efficient the impact of gravitational settling on Helium-depletion is one possible scenario proposed to solve the above mentioned Helium-depletion discrepancy[8].

Overall, the onset of significant Helium-abundance dispersion (in correspondence of the M-jump temperature) and the measured Helium-abundances being anyways larger than expected are both suggestive of the onset of an atmospheric process. The alternating appearance/disappearance of magnetic spots thus provides a viable channel through which randomised enhancement/depletion in Helium are generated. At the same time, the thereby implied presence of *weak* magnetic fields will necessarily trigger some low level of stellar winds that may retard the effects of gravitational settling and, relatively, "increase" the Helium-abundance. Alleged stellar winds in sdBs/EHBs bring about an-

other potential parallelism with young B-type MS stars where chemical peculiarities (such as the $^{3}$He-isotope anomaly and occurrence of Helium rich/poor stars) were linked[9] to similarly *weak* stellar winds and *low* mass-loss rates.

**Modelling of a Stellar Spot:** First, the surface of vEHB-12 in NGC2808 was approximated by a blackbody model with a temperature of $\sim 20,500$ K as derived from the average $(U_{Johnson} - V_{Johnson})$ color. Second, the emission originating from the spot was simulated using a grid of blackbody temperatures varying between 16,500 and 28,500 K, and *contrast ratios* between the star/spot emission were derived using the $U_{Johnson}/R_{Johnson}$ filter transmission curves. The limb darkening quadratic coefficients in the $U_{Johnson}/R_{Johnson}$ filters were obtained from the EXOFAST[10] routine. The light curve simulations were generated using the KSINT software[11] which integrates the total emission from the spotted star, incorporating the full-grid of the spot's properties (longitude/latitude/dimension and temperature). These simulations were later repeated varying the star's inclination angle with respect to the line of sight. We then, simultaneously, fit the *observed* $U_{Johnson}/R_{Johnson}$ light curves to the full-grid of *simulated* models, searching for solutions that minimise the $\chi^2$ residuals and lower the spot's temperature contrast. Figure 3 (in the Main text) shows the best simultaneous modelling of the spot in vEHB-12 and converges on the presence of a single, giant and bright ($\sim 2,500$ K hotter than its surroundings) stellar spot covering as much as $\sim 25\%$ of the EHB surface. The high temperature-contrast estimated for the spot in vEHB-12 is however in line with the trend of increasing spot/surrounding-photosphere temperature-contrast with increasing stellar effective temperature[12]. In particular, whereas typical spots' temperature-contrasts for M-type stars are estimated around $\sim$ 350 K, these reach $\sim$ 1,400 K for G-type stars, and are expectedly higher for B-type stars.

One might be puzzled as to how *all* of our EHB light curves are characterised by single-wave photometric modulation. In this regard, we draw parallels to applications of the oblique rotator model[13] (*i.e. a dipole magnetic field whose axis is tilted with respect to the rotation axis*) that successfully reproduced[14] the *simultaneous* occurrence of single-wave photometric/spectroscopic/magnetic modulation in a $B_P$ Helium-poor HD 21699 star. In principle, it envisages one large Helium-spot around one of the magnetic poles while a Silicon-spot is at the opposite pole. However, and in order to avoid the occurrence of *double-wave* modulation, the dipolar magnetic field necessarily needed to be *off-centre*[15]; i.e. displaced from the star's centre by a given distance (smaller than the stellar radius). The resultant configuration is one in which the two magnetic poles are now *closer* to each other on the stellar surface (unlike that of a *centrally* dipole field where the poles are separated by 180°). The two, *nearby*, poles will then confine *a* single/large spot of, say, Helium-enhanced region, while the Helium-depleted/Silicon-enhanced spot lies on the opposite hemisphere[16].

Although maximum Helium-abundance is expected at the two closely-positioned magnetic poles, these two poles are not actually "resolved". As a result, the Helium-enhanced spot coincides with the poles' *average/intermediate* position. Thus, owing to this *averaging* process over a given hemisphere, *a single* Helium-spot is observed and the overall Helium-abundance is maintained *low*, as for HD 21699. Along these lines, we note that the observed *uvby* single-wave light curves (of a magnetic $B_P$ Helium-rich HD 37776 star[17]) were successfully reproduced, both in shape and amplitude, by introducing ad-hoc enhancement/depletion in surface Helium/Silicon abundances in the observed spectra (aka magnetic spots), later used to recover the correspondent (variable) flux in the *uvby* filters. A similar analysis, assuming other elements of relevance (e.g. Iron/Helium for our EHB variables) is desirable, but requires (currently unavailable) surface chemical composition maps. Lastly, we note

that similarly configured *off-centre* dipolar magnetic fields generally provided[18] a better reproduction of spectroscopic observations for magnetic white dwarfs.

Thus, the modelled giant *bright* spot occupying $\sim 25\%$ of the stellar surface of vEHB-12 (c.f. Fig. 3 of the Main text) would represent a $\sim 3,000$ times scaled-up version of a typical solar dark spot, where the *vertical* magnetic field lines are seen ascending/descending from the poles of the magnetic spot in one hemisphere, while on the opposite hemisphere, the magnetic field lines are predominantly *tangential/horizontal*. This vEHB-12 giant spot configuration, especially that regarding its putative magnetic poles being separated by $\sim 60°$, also implies that the imprint of the ascending/descending vertical/longitudinal magnetic lines will be *washed out* when measuring the *global* longitudinal magnetic field in the visible hemisphere; i.e. reflecting the presence of overall *weak* magnetic fields.

**Why Not All ?** Puzzled by the very similar EHB variable frequency in the 3 GCs we took our simulations a step further and evaluated the *impact* of the stellar spot properties on the recovered EHB variables fraction. In this regard, we first simulated a full-set of models that take into account all possible parameters characterising the stellar spot (i.e. its latitude, dimension, and temperature contrast). Each of these models were then re-generated with different photometric periods and viewing angles of the star. In particular, we employ the same KSINT software used to generate $U_{Johnson}$ filter light curves with stellar spots having: (i) temperature between $17,000 - 24,000$ K, ranging in steps of 250 K; (ii) latitudes between $-90° \div 90°$, ranging in steps of 10°; (iii) angular spot dimensions between $10° \div 90°$, ranging in steps of 10°; (iv) fifty photometric periods randomly selected between $2.0 - 10.0$ days; and (v) stellar inclination angles between $0° \div 90°$ ranging in steps of 10°. These light curves were simulated using our NGC2808 VIMOS time-sampling and typical $U_{Johnson}$ filter photometric errors generated randomly for each simulated light curve, and then re-run through the AoV_HARM algorithm to derive the False-Alarm-Probability and the photometric $U_{Johnson}$ amplitude, as done for the *observed* light curves. Overall, the library of simulated models included a total of 2,167,854 light curves.

The lower limits of the $U_{Johnson}$amplitude and the AoV_HARM false-alarm-probability as determined for the NGC2808 *observed* light curves are $\Delta U_{Johnson} \sim 0.06$ mag and $\sim 10^{-11}$, respectively. The *simulated* light curves that had a *larger* $U_{Johnson}$ amplitude and *lower* false-alarm-probability (than these limits) were selected and their frequency was found to be $\sim 33\%$. This is already a very significant result: assuming a flat distribution - of all possible geometric properties/projections of the stellar spots - would already imply that two-thirds of all simulated models *do not* match the observed (amplitude/false-alarm-probability) properties. In particular, the recovery of $\sim 33\%$ should be considered as an *upper limit* because the library of modelled light curves does not take into account the *real* (and unknown) distribution of the spot's physical properties. This is to say that, for the time being, we do not know of any *preferential* dimension/latitude distributions (e.g. preferential latitude location of spots and spot cycles as in our Sun) of the stellar spots. Thereby all these values are considered equally possible, and their impact is hardly accountable for. On the other hand, the distribution of the spot's temperature contrast ($\Delta T$) is *unlikely* to be a random function, because quite simply the observed EHB variables showing the highest $U-$amplitudes are a minority. We therefore make the reasonable assumption that the underlying distribution of the spot's $\Delta T$ is not-flat and (as compared to the star's average temperature fixed at 20,500 K in all simulations) follows a Gaussian function with a standard deviation $\sigma$ that is anywhere between $500 \div 2,500$ K. Assuming the aforementioned Gaussian function and realising 1,000 experiments (each including 94 light curves

as our reference EHB sample) for a given $\sigma$ we derive the frequency of the simulated light curves satisfying our measurement constraints. We find that the best re-production of the properties of our EHB variables is obtained with a $\sigma = 1,000$ K Gaussian distribution that includes (at a $\sigma \sim 2.2$ level) the $\Delta T \sim 2,500$ K estimated for vEHB-12, which is our largest amplitude variable. Granted the above, we infer that the frequency of the spotted/simulated light curves that satisfies our observed constraints could go down to $\sim 12.3 \pm 3.7\%$. This is surprisingly similar to the observed frequency. Many unknowns can alter this estimate (e.g. the presence of more than one spot, the eventual geometrical distribution of these multiple spots, etc). However, any further sophistication of our first-order simulations is likely to introduce uncertainties of its own. The above simulations clearly indicate that the spots' specific properties heavily affect the detectable variability fraction. Overall, the observed EHB variable frequency $\sim 12 - 15\%$ in the 3 GCs is yet compatible with the spot phenomenon being a wide-spread feature, lurking at some level, among these certainly chemically peculiar EHB stars.
Lastly, we emphasise that the above simulations (and the important implications they deliver) were made possible thanks only to the availability of a, sizeable, homogeneous EHB sample (sharing basically the same distance, age, and metallicity) monitored by a single photometric survey (with known photometric precision, depth and completeness). Similar procedures are hardly applicable to field sdBs *sparsely* distributed in the Milky Way field subject to intrinsic uncertainties in distance, reddening, age, and original MS chemical composition.
**The Padua EHB variables:** Supplementary Fig. 5 displays the light curves of the remaining six, aperiodic, EHB (*Padua*) variables. NGC6752 is the only cluster for which we could integrate our 3-year data with existing 6-year archival data. The case of *Padua-7* is quite instructive: once a luminosity transition has taken place (in about 400−500 days) the EHB star displayed an overall consistent luminosity for the following $\sim$ 4 years; belying a "constant" star profile. Thus, *only* long-term, high-precision, regular monitoring can reveal the presence of *Paduas*, and we suspect more of them exist not just in NGC6752 but in other GCs as well. Gaia proper-motion determinations of the *Padua* variables and spectra of *Padua-1/7* establish a firm NGC6752 membership.
The origin of the *Padua* variability is unlikely due to some peculiar evolutionary scenarios (e.g. Late Thermal Pulses[19,20]). Indeed, the estimated temperature evolution of *Padua-1*, as due to the $u_{SDSS} - r_{SDSS}$ colour transition in the arc of six years, is $\lesssim 200$ K. This is *too slow* for "born again" scenarios involving *rapid* evolution lasting *only* for decades. An additional piece of evidence supporting this conclusion is found when reviewing the position of these long-term EHB variables in color-magnitude diagrams collected decades ago. Identification of Padua-1/2 and 5 in the 1980 $B/V$ photographic plates[21] still reflected typical EHB colors/luminosities. We also exclude the possibility that *Padua-1* variability is due to pulsation, at any short-term regime. In particular, we preclude scenarios like *Blue Large-Amplitude Pulsator* (BLAP[22]: hot sdB showing RR Lyrae-like variability with $\sim 20-40$ minute periods). In this regard, we availed $\sim$ 3.5 hours of continuous UltraCAM[23] $20_{sec}$ $u_{SDSS}$ filter fast-photometry (programme 0103.D-0158, P.I. L. Monaco). Periodogram analysis of the same ultraviolet data showed no significant peaks for pressure-mode oscillations between $100 - 300$ seconds.
A close-binary origin is also unlikely. Six spectra of *Padua-1* were collected on the night of November $23^{rd}$ 2018 at the Low Dispersion Survey Spectrograph (LDSS-3), mounted at the Magellan Clay telescope (Chile). The VPH-Blue grism provided a wavelength coverage between $\sim 3800 - 6200$ Å and a resolution of $\sim$ 1900. The $6 \times 600_{sec}$ successive spectra were reduced as in Methods 2. These provided a radial velocity RMS of $\sim$ 11 km/s with respect to the estimated $\sim$ 13 km/s error on single

measurements, suggesting that *Padua-1* is *unlikely* a member of a very-close binary. Similarly, the 6 FLAMES spectra of *Padua-7* (presented in Methods 2) collected over a period of 8 days provided a radial velocity RMS of ~ 4 km/s, very close to the ~ 3 km/s associated error for a given measurement. Combined, the *Padua-1/7* radial velocity monitoring disfavour close-binary systems up to periods of few days. One last piece of evidence arguing against a possible binary origin is found in the estimated energetics of the Padua-1 superflare ($10^{39-40}$ erg). Such levels are much higher than those typically occurring in WD/M-type binary systems[24] (where the flaring event has been associated to an active/cool M-type dwarf). Indeed, had the *Padua-1* superflare been due to a hidden faint/cool K/M-type companion the flare energy would have been orders of magnitudes higher than the strongest flares ever measured in *isolated* K/M-type dwarfs[25]. In conclusion, the *Padua* variables are not pulsators nor members of binary systems.

Granted the above, there is a notable similarity of the form of the *Padua-1* superflare with the occurrence[26,28] of similar outbursts in cool ($T_{eff} \sim 10,900 \pm 300$ K) and pulsating (periods of ~ 1000 seconds) field WDs . With respect to the single/long superflare event in *Padua-1*, the outbursts in these cool/pulsating WDs display[27] a very high re-occurrence frequency of once every ~ 5 days, a short average duration of ~ 12 hours, a slightly higher amplitudes ~ 10%, and much lower energetics ~ $10^{33}$ erg. Despite these difference, it is interesting to note the very restricted temperature regime of these outbursting WDs (basically coinciding with the G-jump[29]) and its coincidence with the onset of superficial convection by the Hydrogen convection zone (sought[27] to drive the gravity-mode pulsation). In particular, the outbursts are modeled as a "*temporary, rapid re-assignment of kinetic energy away from pulsation*[26]". In this regard, we note that the same scenario we use to explain the occurrence of EHBs' magnetic spots also accommodates for the occurrence of *Padua-1*. In particular, it envisages a "build-up of magnetic energy" but within the hotter sub-surface HeIICZ or in the radiative layer above it[3]. Thus, the "turbulent" effects of the HeIICZ and HCZ, both being so close to the surface (or actually onsetting convective photospheres as in the WDs pulsators) bring about an interesting EHB/WD parallelism. However, the UltraCAM fast photometry of *Padua-1* did not reveal any significant pulsation signature, marking a clear difference with the outbursting/pulsating WDs at $T_{eff} \sim 10,900 \pm 300$ K. Future observational/theoretical investigations are needed to shed more light on the occurrence of outbursting/flaring events and the role played by the surface/sub-surface Hydrogen/Helium convective layers.

**$\alpha^2$ CVn/Magnetism in Galactic Field sdBs:** One might wonder why the EHB spot-induced $\alpha^2$ CVn rotational variability in GCs has not been detected in the Galactic field sdB counterparts, despite the latter being subject of many surveys. In principle, there is no *a priori* reason for which the EHB field-counterparts *should not* display $\alpha^2$ CVn variability. Indeed, Galactic field sdB (as GC EHB stars) display the same complex enhancement/depletion chemical anomalies attributed to diffusion effects (i.e. chemically peculiar). Hence, we argue that the apparent lack of $\alpha^2$ CVn variability detection in field sdB is likely due to it being hampered by, other, specific sdB properties. For example, with a frequency of ~ 50%[30], the preferential sdB close-binary evolution of the two components is likely to dominate/conceal the lower-amplitude $\alpha^2$ CVn variability in the light curves. Moreover, eventual tidally-locked components (stellar rotation is synchronised with the orbital period) is likely to induce faster-rotation of the components and shift the $\alpha^2$ CVn variability to shorter-periods. Overall, and with respect to EHBs in GCs, the sdBs' much-higher binary fraction, their significantly-lower age and relatively-higher metallicity[31] (the latter likely implying differences in stellar spots sizes and

contrast[32]) are all factors possibly contributing in smearing the signature of $\alpha^2$ CVn variability in field sdBs.

In this regard, space-based surveys probe the millimagnitude variability regime and allow deeper examination of eventual detection of $\alpha^2$ CVn variability in field sdBs. We bring to the attention the case of CD-38 222, holding TESS[33] serial number 118327563. The physical parameters[25,34] of this star ($T_{eff} \simeq 26,300$ K, $log\, L/L_{\odot} = 1.42$ and $log\, g = 5.5$) place it perfectly in the EHB segment, just hotter than the M-jump. CD-38 222, one of the few cases of an apparently[35] *single* sdB. It was concluded[25] to display rotational variability with a period of $\sim 0.229$ days and semi-amplitude of less than one part per thousand (as seen in the upper panel in Supplementary Fig. 6. Such low-levels of variability amplitudes can easily escape detection in ground-based surveys[32,36], but are perfectly in line with *all* sdBs being chemically peculiar, easily accommodating for the presence of superficial inhomogeneities upon their surface, i.e. spots. Indeed, CD-38 222 is the *first*[35] Galactic field sdB showing *Helium vertical-stratification* (which could be modeled[14] as due to Helium-enhancement at the magnetic poles of a Helium-spot, as explained in Supplementary Information 1). The extremely low-amplitude variability detected in CD-38 222, *possibly* a representative of the $\lesssim 20\%$ minority of *single* sdB stars, is probably suggestive of how/why $\alpha^2$ CVn variability is apparently lacking among field sdBs.

While definitive evidence indicates that CD-38 222 is not a member of a *close-binary* system, there remains a suggestion[36] it might hide a faint K-type companion in a wide-orbit. However, the high energetics of the superflare in CD-38 222 makes it unlikely that the K-type dwarf is the source of the superflare. Indeed, a hypothetical superflare in the K-type dwarf would imply energetics that are orders of magnitude stronger than those typically measured in isolated flaring K/M-type dwarfs[25]. One final piece of evidence unambiguously supporting the *single-sdB* star nature of CD-38 222 is provided when assuming that the $\sim 0.22$-day light modulation is due to a rotating spot on the $\sim 0.25\,R_{\odot}$ (as inferred from its luminosity/temperature). This delivers a rotational velocity of $\sim 55.5$ km/s in excellent agreement (considering all sources uncertainties) with two estimates of the projected rotational velocities of $\sim 48.0$ and $\sim 58.0$ km/s, respectively derived from metal and Helium line profiles[36].

CD-38 222 is perhaps a unique case of an sdB also showing the presence of a superflare[25] event (releasing up to $\sim 10^{35}$ erg, thousand times more energetic than those occurring in the Sun). This superflare event necessarily implies the presence of an underlying magnetic field in the sdB. Most interestingly, the magnetic field of CD-38 222 has been investigated twice[34,37] only to conclude it being confined to below $\sim 400$ Gauss, i.e. below the significance detection-levels of current top-level instrumentations. Thus, by all means, the presence of a low-intensity magnetic field in CD-38 222 *is* certain, regardless of it being detected or not. This is particularly relevant as it lends support to our conclusions on the detected EHB variability and therein presence of similar, low-intensity, magnetic fields. In conclusion, CD-38 222 paves the way for the detection of spot-induced $\alpha^2$ CVn variability and superflare events in field sdBs, as we have established here for GCs EHBs. Clearly, statistically significant sdB/EHB samples are mandatory before a comparative analysis (e.g. differences in flare duration/energies and $\alpha^2$ CVn periods/amplitudes) can be performed.

It is probably too early to evaluate the wider implications of universal magnetism among GCs' EHBs and field's sdBs. This is specially true considering that the matrix managing the formation of EHBs in GCs is rather complex (interplay between cluster's age, cluster's central concentration, Helium-enrichment and mixing, CNO abundance, stellar rotation, and extreme mass-loss) whereas that gov-

erning the sdBs formation is restricted to *binarity* ($\sim$ 80% are *currently* in binaries while the remaining $\sim$ 20% are merger products of *past* binary evolution). One notes that binary evolution is not even considered as a formation channel for EHBs in GCs. In this regard, we cannot help but notice that the only sdB star showing both $\alpha^2$ CVn variability and superflare event (and very likely a *single-star*) is also known for a relatively high rotation velocity. The latter is often used as a signature of merger events, and overall there are suggestions that stellar mergers are likely related to a strong magnetic phenomenon[38]. This opens to the remote (but not to be excluded) possibility that the *entirety* of EHBs in GCs can be by-products of stellar mergers. Interestingly, this possibility has been validated by simulations[39] showing that the (WD/WD) merger channel - in stellar systems older than $\sim$ 8 Gyr - is expected to dominate the (Roche lobe overflow and the common-envelope) channels and form more than $\geq$ 50% of the total EHB fraction in a typical GC. In this regard, the rather high stellar density in GCs (*continuously* favouring encounters/mergers) and the fact that the EHB stars share basically the same distance/reddening/metallicity (i.e. reducing to the minimum temperature/gravity uncertainties) provide the ideal benchmark where one can identify merger-products among EHB stars. Unfortunately, the homogeneous properties of EHBs *currently* show no evidence of any discernible outliers (e.g. larger masses, faster rotation, brighter luminosities, or peculiar red-excess) enabling one to pinpoint a merger by-product in EHBs samples. Ultimately, the merger scenario is left unverified.

$\alpha^2$ **CVn/Magnetism in Galactic Field WDs:** Despite the common use of WDs as photometric/spectroscopic standards, reports of the presence of stellar spots and related variability date back to the seventies[40,41]. Nowadays, frequent detection of both bright/dark spot-induced photometric variability (on hours-to-day timescales) is reflecting considerably large frequencies ($\sim$ 50%[42] and $\sim$ 67%[43]). Focusing our attention on hot WDs (close to our $\sim 20,000 - 30,000$ K EHB variability regime) we recall WDs characterised by Hydrogen/Helium dominated atmospheres (i.e. DA with $T_{eff} \geq 13,000$ K and DB with $23,000 \leq T_{eff} \leq 28,000$ K, respectively) are both expected to display *fully-radiative* envelopes (as do our EHBs, field B-type and $B_P$ stars). Invoking stellar-spots for cooler WDs with convective atmospheres[44] is, relatively, an easy task (i.e. the hypothesised magnetic fields would inhibit surface convection and naturally form a cooler/darker spot, as is in our Sun). On the other hand, the origin of the photometric variability of hotter/radiative WDs (e.g. LB8915, PG165+441, GD 394 and other 5 cases[42]) remains a mystery[43]. Indeed, conventional (Sun-like) spots cannot be invoked nor formed upon such hot/radiative-enveloped WDs, and magnetic fields (whenever estimated/detected) are apparently not sufficiently strong-enough (at least in the WDs nomenclature) to introduce measurable photometric variability. The case of the $\sim 35,000 - 39,000$ K, Hydrogen-rich, GD 394 is particularly emblematic. Given its apparently single-star status[45] and estimated upper-limit $\sim 12,000$ Gauss magnetic field (would be considered a rather *extremely-weak* field in the WDs context), it is utterly hard to explain its remarkable Far-Ultraviolet, single-wave, variability with $\sim$ 1.15 day period and $\sim$ 25% amplitude variations. However, its atmosphere is almost certainly radiative and, not-surprisingly, the most likely scenario for its Far-UV variability is one envisaging inhomogeneous surface abundance distribution of metals[45] (aka Far-UV dark/circular spot). This, in principle, is accommodated for by invoking the presence of a, weak, magnetic field.

Many scenarios are put forward to explain the WDs variability[42] and, leaving aside the obvious ones arising due to binary evolution (e.g. transit, beaming, reflection and thermal emission from a close-companion) it all comes down to different shades of a single scenario that combines the WD rotation with “non-uniform surface emission”[42]. In particular, it is interesting to note how the alleged

WDs *surface inhomogeneities* remain the common, fundamental ingredient of apparently "different" modelings[42]; these being cool/dark magnetic spots, hot/bright spots formed due to accretion of ISM material, magnetic dichroism, and most interestingly, non-uniform Far-UV line opacity absorption resulting in optical/near-IR fluorescence. Indeed, the latter scenario was concluded[42] to be the only one that is applicable/viable to *all cases* of variability among WDs (regardless of their envelope structure), and not surprisingly its fundamentals *reflect* what we assume to be the definition of a "magnetic spot" in EHBs. In this regard, the scenario hypothesised for our EHBs (*weak* magnetic fields that do not introduce Zeeman splitting and yet reach the stellar radiative surface) are likely to afflict the temperature of the WD *radiative photosphere* and trigger magnetic spots. In particular, since the optical depth of the WD/EHB photosphere is expectedly *lower* in the magnetic spot surrounding (as due to the contribution of magnetic pressure) it provides a deeper glimpse of the *hotter* stellar interior (i.e. hot/bright magnetic spot)[3].

# Supplementary Figures

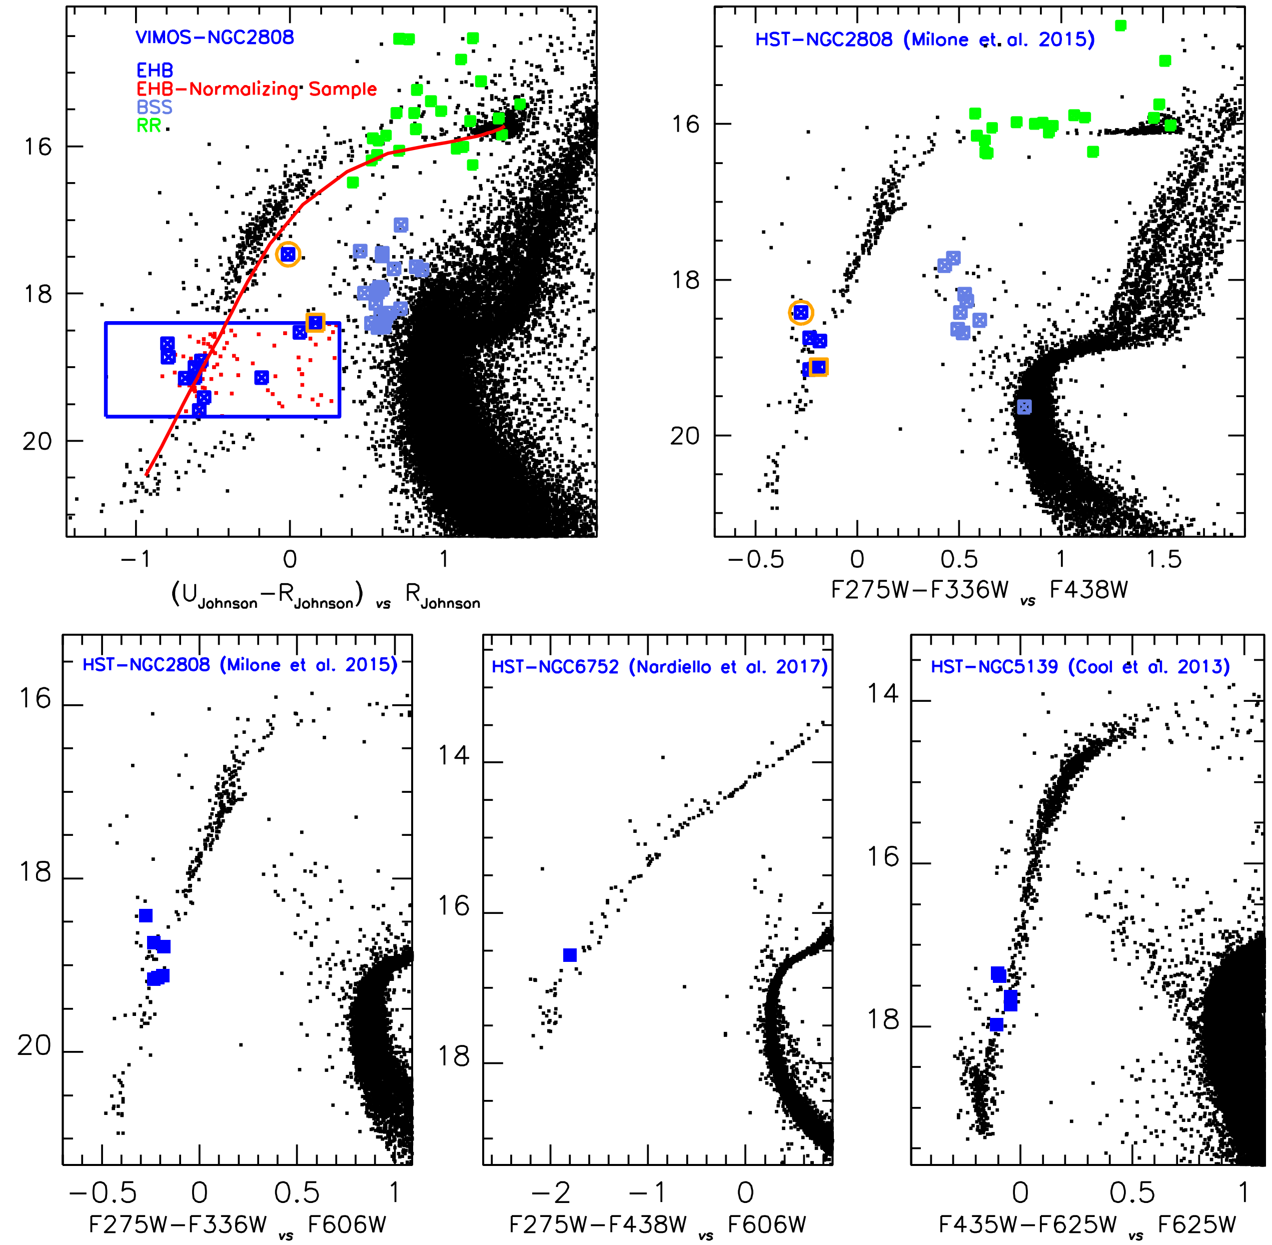


Supplementary Figure 1: Estimating the EHB variable frequency. Upper-left panel displays our NGC2808 VIMOS diagram highlighting all identified variables, the box delimits the EHB sample used to normalise the EHB variables frequency while a ZAHB model is used to confirm the EHB variables temperature range ($\sim 17,500$–$24,500$ K). The two EHB variables with open orange symbols are *confirmed* EHB stars, as identified in the higher resolution HST catalog (upper-right panel). Lower panels show the position of all EHB variables identified in HST diagrams.

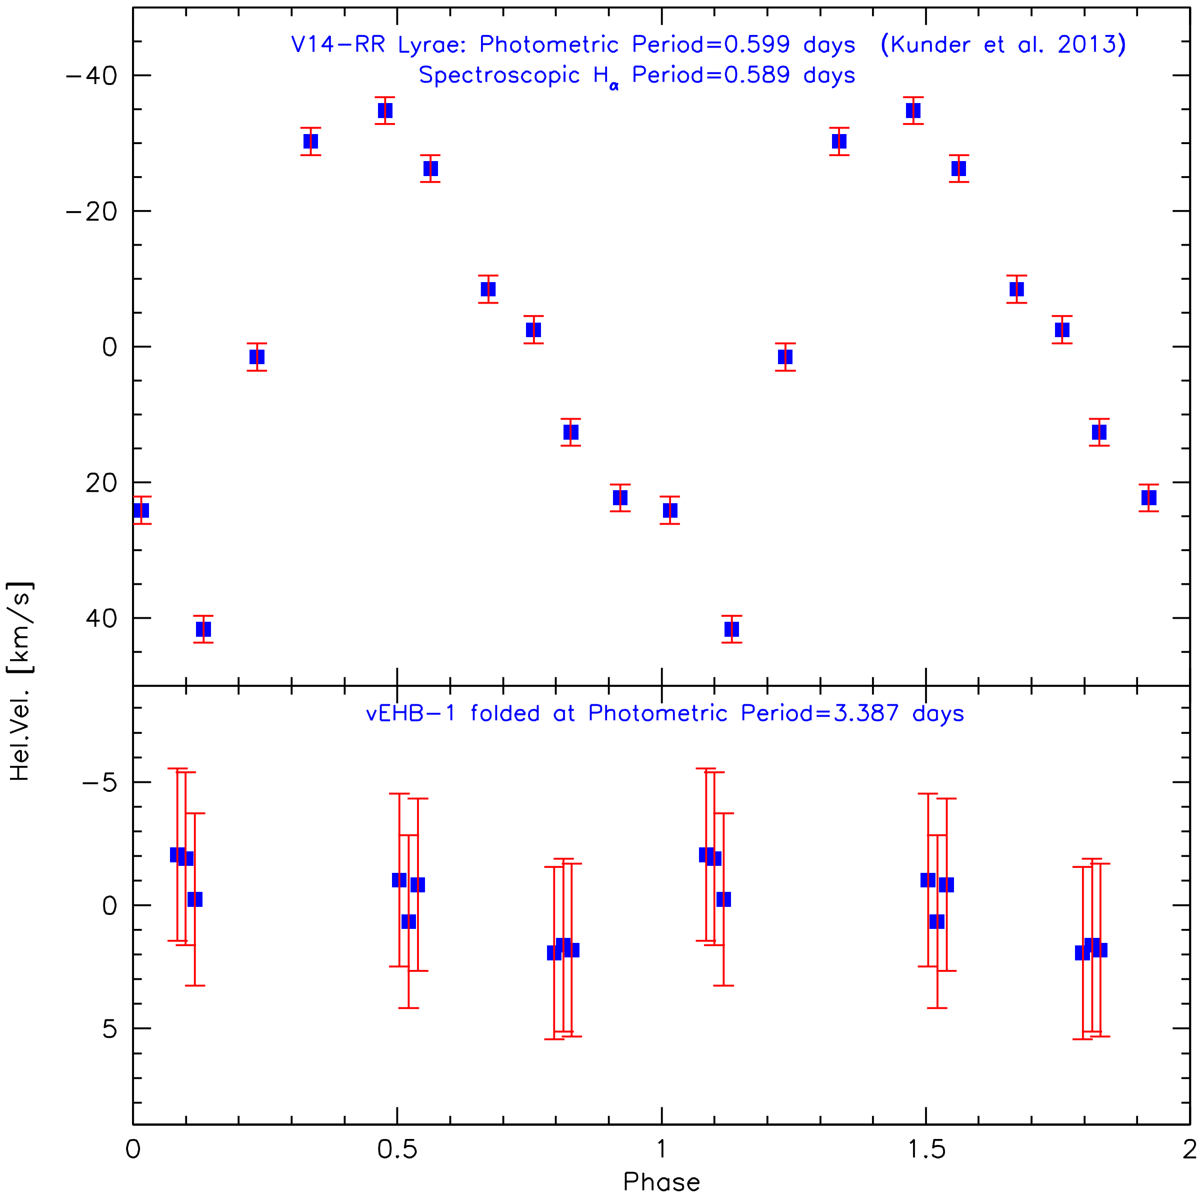


Supplementary Figure 2: No binarity signature detected in the NGC2808 vEHB-1 variable. Upper panel displays the phased $H_\alpha$ radial velocity curve of a *comparison* RR Lyrae star proving a successful detection of velocity variations in the data-set. The lower panel displays the velocity curve of our photometric variable vEHB-1 present in the same data-set. The error bars display the $1-\sigma$ error ($\sim$ 3.5 km/s) estimated at the vEHB-1 luminosity. No significant velocity variations for vEHB-1 are observed. For clarity, the NGC2808 average radial velocity has been subtracted.

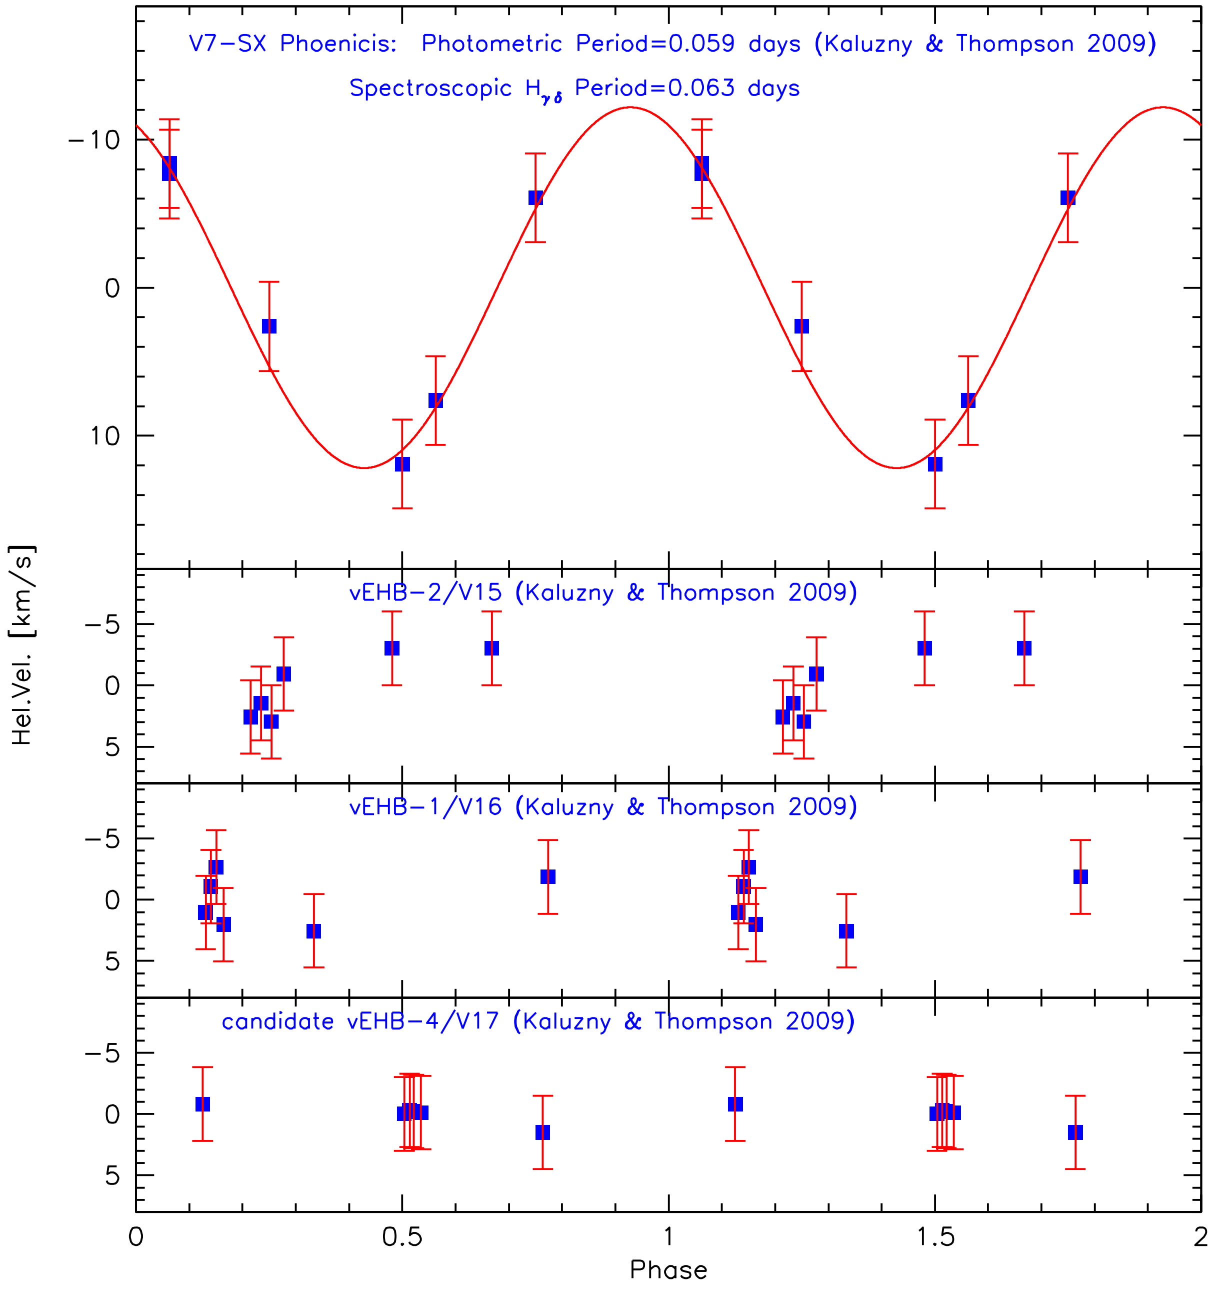


Supplementary Figure 3: No binarity signature detected in the NGC6752 vEHB-1/2 variables. Upper panel displays the phased $H_{\gamma\delta}$ radial velocity curve of a *comparison* SX Phoenicis star[46] proving a successful detection of velocity variations in the data-set. The lower panels display the velocity curves of the 2 EHB photometric variables (and the candidate EHB photometric[46] variable vEHB-4/V17) present in the same data-set. The error bars display the $1-\sigma$ error ($\sim 3.0$ km/s) estimated at the vEHB-1 luminosity. No significant velocity variations for the vEHB-1/2 are observed. For clarity, the NGC6752 average radial velocity has been subtracted.

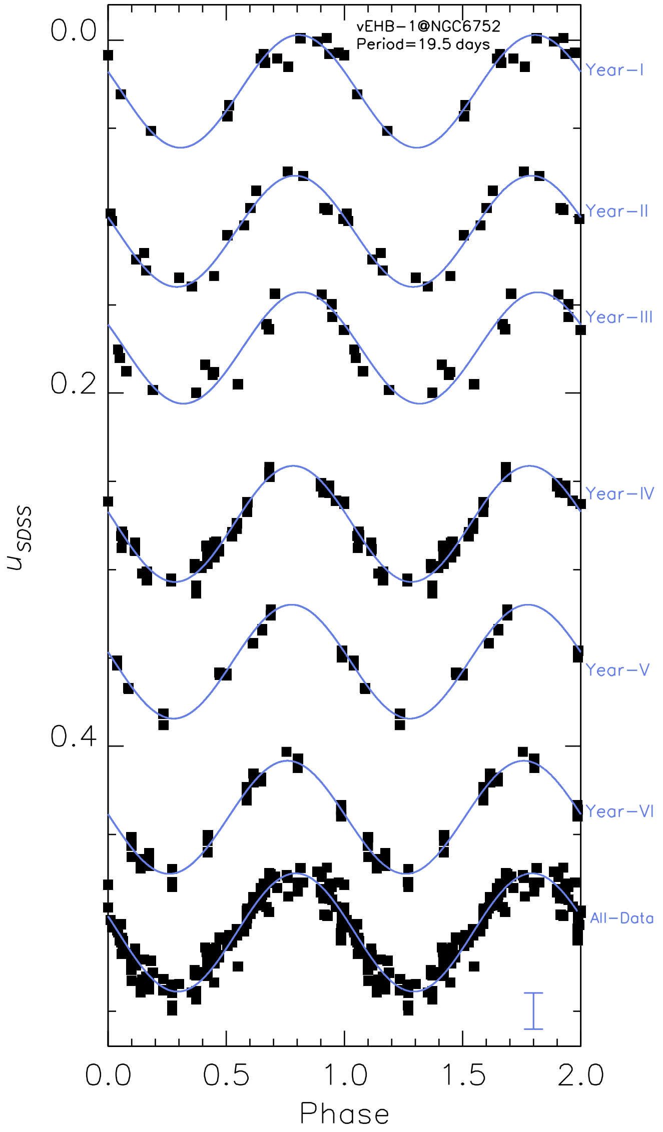


Supplementary Figure 4: The long-term stable variability of vEHB-1 in NGC6752. Bottom plot shows *all* the $u_{SDSS}$ OmegaCAM measurements of vEHB-1 collected over a six-year period. The upper plots show the phased light curves sub-divided over six years. A typical $1-\sigma$ photometric error bar is plotted. The solid light-blue line is the best fitting model (Period$\simeq$ 19.5 days) calculated using the six years' measurements.

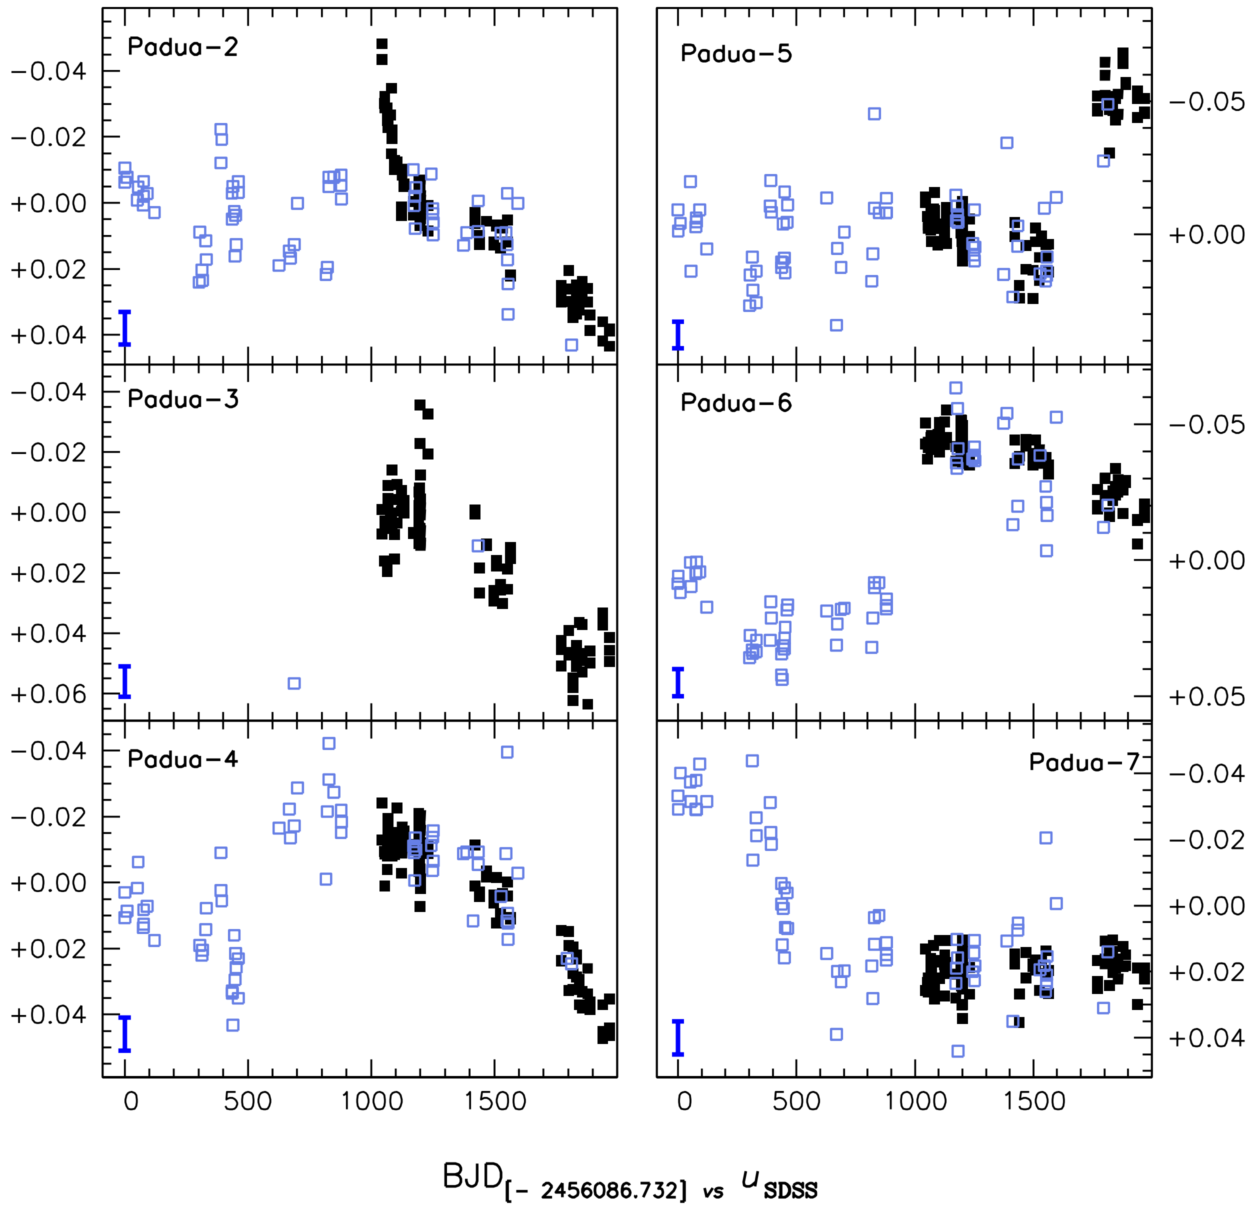


Supplementary Figure 5: The aperiodic long-term *Padua* variables in NGC6752. Light blue squares display the six-year archival OmegaCAM@VST data, while black squares display those originating from our three-year monitoring. A typical $1-\sigma$ photometric error bar is plotted. The *Padua-2* mini-burst is incomplete but discernible.

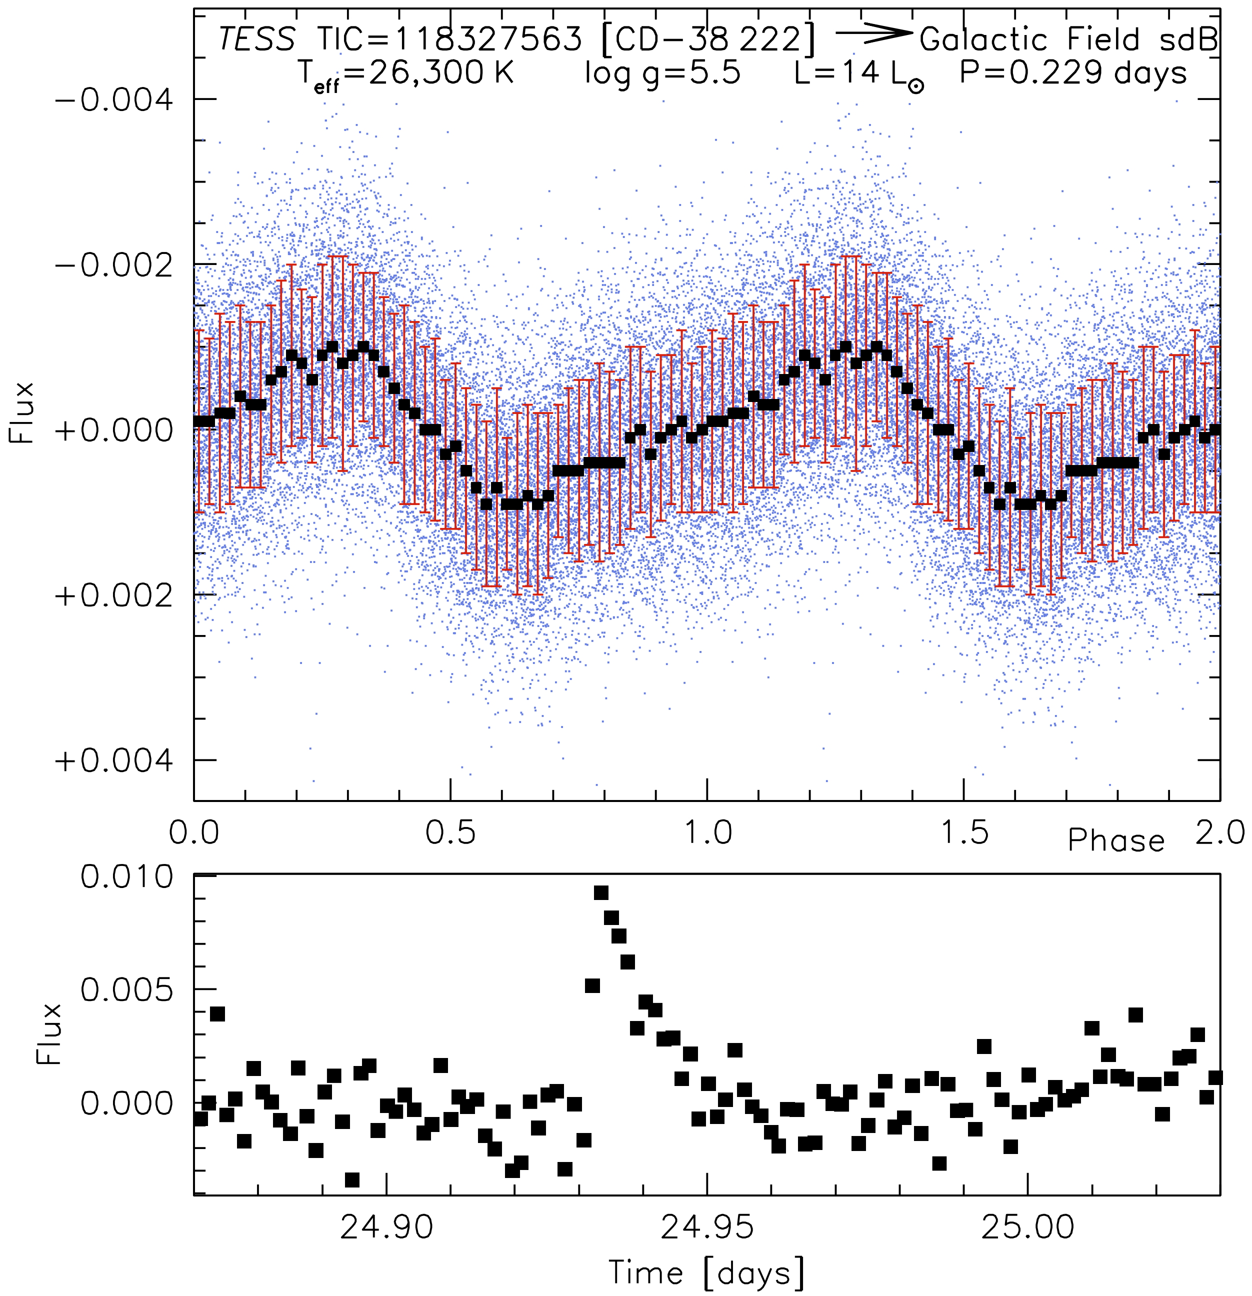


Supplementary Figure 6: Rotational variability and superflare event in a Galactic field sdB. Upper panel displays the folded TESS light curve of a Galactic field sdB showing $\alpha^2$ CVn spot-induced variability. Filled squares are the $2.5-\sigma$ clipped median values every 300 data-points, while the error bars reflect the $1-\sigma$ rms of the clipped Flux values. Lower panel proves the occurrence of an energetic ($\sim 10^{35}$ erg) super-flare event in this field sdB. Both phenomenon necessitate the presence of magnetic fields.

1. Strassmeier, K. G. Starspots. *Astron. Astrophys. Rev.* **17**, 251-308 (2009).

2. Recio-Blanco, A., Piotto, G., Aparicio, A., & Renzini, A. Rotation of Hot Horizontal-Branch Stars in the Globular Clusters NGC 1904, NGC 2808, NGC 6093, and NGC 7078. *Astrophys. J. Lett.* **572**, L71-L74 (2002).

3. Cantiello, M., & Braithwaite, J. Envelope Convection, Surface Magnetism, and Spots in A and Late B-type Stars. *Astrophys. J.* **883**, 106 (2019).

4. Brown, T. M., et al. The Hubble Space Telescope UV Legacy Survey of Galactic Globular Clusters. VII. Implications from the Nearly Universal Nature of Horizontal Branch Discontinuities. *Astrophys. J.* **822**, 44 (2016).

5. Groth, H. G., Kudritzki, R. P., & Heber, U. Photospheric convection zones and evolution of subluminous OB-stars. *Astron. Astrophys.* **152**, 107-116 (1985).

6. Michaud, G., Richer, J., & Richard, O. Horizontal branch evolution, metallicity, and sdB stars. *Astron. Astrophys.* **529**, A60 (2011).

7. Moni Bidin, C., et al. Spectroscopy of horizontal branch stars in $\omega$ Centauri$\star$. *Astron. Astrophys.* **547**, A109 (2012).

8. Unglaub, K. Mass-loss and diffusion in subdwarf B stars and hot white dwarfs: do weak winds exist?. *Astron. Astrophys.* **486**, 923-940 (2008).

9. Babel, J. The fading of radiatively driven winds in B stars. *Astron. Astrophys.* **309**, 867-878 (1996).

10. Eastman, J., Gaudi, B. S., & Agol, E. EXOFAST: A Fast Exoplanetary Fitting Suite in IDL. *Publ. Astron. Soc. Pac.* **125**, 83 (2013).

11. Montalto, M., et al. Improvements on analytic modelling of stellar spots. *Mon. Not. R. Astron. Soc.* **444**, 1721-1728 (2014).

12. Panja, M., Cameron, R., & Solanki, S. K. 3D Radiative MHD simulations of starspots. arXiv e-prints arXiv:2003.09656 (2020).

13. Stibbs, D. W. N. A study of the spectrum and magnetic variable star HD 125248. *Mon. Not. R. Astron. Soc.* **110**, 395 (1950).

14. Shavrina, A. V., et al. Spots structure and stratification of helium and silicon in the atmosphere of He-weak star HD 21699. *Mon. Not. R. Astron. Soc.* **401**, 1882-1888 (2010).

15. Stift, M. J. A non-axisymmetric rigid rotator model for magnetic stars.. *Mon. Not. R. Astron. Soc.* **172**, 133-139 (1975).

16. Glagolevskij, Y. V., & Chuntonov, G. A. Composite model for the magnetic field of HD 21699. *Astrophys.* **50**, 362-371 (2007).

17. Krtička, J., Mikulášek, Z., Zverko, J., & Žižňovský, J. The light variability of the helium strong star HD 37776 as a result of its inhomogeneous elemental surface distribution. *Astron. Astrophys.* **470**, 1089-1098 (2007).

18. Kawka, A. Clues to the origin and properties of magnetic white dwarfs. arXiv e-prints arXiv:2001.10672 (2020).

19. Schoenberner, D. Asymptotic giant branch evolution with steady mass loss.. *Astron. Astrophys.* **79**, 108-114 (1979).

20. Iben, I. On the frequency of planetary nebula nuclei powered by helium burningand on the frequency of white dwarfs with hydrogen-deficient atmospheres.. *Astrophys. J.* **277**, 333-354 (1984).

21. Buonanno, R., et al. The giant, asymptotic and horizontal branches of globular clusters. III. Photographic photometry of NGC 6752.. *Astron. Astrophys. Suppl.* **66**, 79-109 (1986).

22. Pietrukowicz, P., et al. Blue large-amplitude pulsators as a new class of variable stars. Nature Astronomy **1**, 0166 (2017).

23. Dhillon, V. S., et al. ULTRACAM: an ultrafast, triple-beam CCD camera for high-speed astrophysics. *Mon. Not. R. Astron. Soc.* **378**, 825-840 (2007).

24. Østensen, R. H., et al. First Kepler results on compact pulsators - I. Survey target selection and the first pulsators. *Mon. Not. R. Astron. Soc.* **409**, 1470-1486 (2010).

25. Balona, L. A., et al. Rotational modulation in TESS B stars. *Mon. Not. R. Astron. Soc.* **485**, 3457-3469 (2019).

26. Hermes, J. J., et al. A Second Case of Outbursts in a Pulsating White Dwarf Observed by Kepler. *Astrophys. J. Lett.* **810**, L5 (2015).

27. Bell, K. J., et al. The First Six Outbursting Cool DA White Dwarf Pulsators. In *Proceedings of the 20st European Workshop on White Dwarfs*, **509**, 303 (2017).

28. Bell, K. J., et al. KIC 4552982: Outbursts and Asteroseismology from the Longest Pseudo-continuous Light Curve of a ZZ Ceti. *Astrophys. J.* **809**, 14 (2015).

29. Grundahl, F., Catelan, M., Landsman, W. B., Stetson, P. B., & Andersen, M. I. Hot Horizontal-Branch Stars: The Ubiquitous Nature of the "Jump" in Strömgren u, Low Gravities, and the Role of Radiative Levitation of Metals. *Astrophys. J.* **524**, 242-261 (1999).

30. Deca, J., et al. PG 1018-047: the longest period subdwarf B binary. *Mon. Not. R. Astron. Soc.* **421**, 2798-2808 (2012).

31. Latour, M., et al. A Helium-Carbon Correlation on the Extreme Horizontal Branch in $\omega$ Centauri. *Astrophys. J.* **795**, 106 (2014).

32. Paunzen, E., et al. Search for stellar spots in field blue horizontal-branch stars. *Astron. Astrophys.* **622**, A77 (2019).

33. Ricker, G. R., et al. Transiting Exoplanet Survey Satellite (TESS). *Journal of Astronomical Telescopes, Instruments, and Systems* **1**, 014003 (2015).

34. Landstreet, J. D., Bagnulo, S., Fossati, L., Jordan, S., & O'Toole, S. J. The magnetic fields of hot subdwarf stars. *Astron. Astrophys.* **541**, A100 (2012).

35. Schneider, D., Irrgang, A., Heber, U., Nieva, M. F., & Przybilla, N. NLTE spectroscopic analysis of the $^3$He anomaly in subluminous B-type stars. *Astron. Astrophys.* **618**, A86 (2018).

36. Geier, S., et al. The subdwarf B star SB 290 - A fast rotator on the extreme horizontal branch. *Astron. Astrophys.* **551**, L4 (2013).

37. Bagnulo, S., Fossati, L., Landstreet, J. D., & Izzo, C. The FORS1 catalogue of stellar magnetic field measurements. *Astron. Astrophys.* **583**, A115 (2015).

38. García-Berro, E., et al. Double Degenerate Mergers as Progenitors of High-field Magnetic White Dwarfs. *Astrophys. J.* **749**, 25 (2012).

39. Han, Z. A possible solution for the lack of EHB binaries in globular clusters. *Astron. Astrophys.* **484**, L31-L34 (2008).

40. Landi Degl'Innocenti, E. Are there spots on magnetic white dwarfs? *Astrophys. J.* **209**, 208-213 (1976).

41. Sion, E. M., Schaefer, K. G., Bond, H. E., Saffer, R. A., & Cheng, F. H. Hubble Space Telescope Observations of an Accreted Silicon SPOT on the White Dwarf in V471 Tauri. *Astrophys. J. Lett.* **496**, L29-L32 (1998).

42. Maoz, D., Mazeh, T., & McQuillan, A. Kepler and the seven dwarfs: detection of low-level day-time-scale periodic photometric variations in white dwarfs. *Mon. Not. R. Astron. Soc.* **447**, 1749-1760 (2015).

43. Brinkworth, C. S., Burleigh, M. R., Lawrie, K., Marsh, T. R., & Knigge, C. Measuring the Rotational Periods of Isolated Magnetic White Dwarfs. *Astrophys. J.* **773**, 47 (2013).

44. Kilic, M., et al. A Dark Spot on a Massive White Dwarf. *Astrophys. J. Lett.* **814**, L31 (2015).

45. Dupuis, J., Chayer, P., Vennes, S., Christian, D. J., & Kruk, J. W. Adding More Mysteries to the DA White Dwarf GD 394. *Astrophys. J.* **537**, 977-992 (2000).

46. Kaluzny, J., & Thompson, I. B. Variable Stars in the Globular Cluster NGC 6752. *Acta Astron.* **59**, 273-289 (2009).

47. Momany, Y., et al. A New Feature along the Extended Blue Horizontal Branch of NGC 6752. *Astrophys. J. Lett.* **576**, L65-L68 (2002).

48. Momany, Y., et al. The ubiquitous nature of the horizontal branch second U-jump. A link with the Blue Hook scenario?. *Astron. Astrophys.* **420**, 605-617 (2004).

49. Milone, A. P., et al. The Hubble Space Telescope UV Legacy Survey of Galactic Globular Clusters. III. A Quintuple Stellar Population in NGC 2808. *Astrophys. J.* **808**, 51 (2015).

50. Moni Bidin, C., Villanova, S., Piotto, G., & Momany, Y. A lack of close binaries among hot horizontal branch stars in globular clusters. II. NGC 2808. *Astron. Astrophys.* **528**, A127 (2011).

51. Nardiello, D., et al. The Hubble Space Telescope UV Legacy Survey of Galactic Globular Clusters - XVII. Public Catalogue Release. *Mon. Not. R. Astron. Soc.* **481**, 3382-3393 (2018).

52. Cool, A. M., et al. HST/ACS Imaging of Omega Centauri: Optical Counterparts of Chandra X-Ray Sources. *Astrophys. J.* **763**, 126 (2013).

53. Moehler, S., et al. The hot horizontal-branch stars in $\omega$ Centauri. *Astron. Astrophys.* **526**, A136 (2011).

54. Latour, M., Randall, S. K., Calamida, A., Geier, S., & Moehler, S. SHOTGLAS. I. The ultimate spectroscopic census of extreme horizontal branch stars in $\omega$ Centauri. *Astron. Astrophys.* **618**, A15 (2018).

Table 1: The measured J2000 coordinates and Johnson-$UBV$ magnitudes of the EHB variables in NGC2808, NGC6752[47] and NGC5139[48], respectively. The last four columns report the distance (in arcmin) from the GC centre, the derived period, the full-amplitude as measured in the ultraviolet-filter ($U_{Johnson}$ for NGC2808 and $u_{SDSS}$ for NGC6752 and NGC5139) and, when available, information regarding their temperature, radial velocity monitoring, and presence in HST catalogs.

| ID | Ra | Dec | U | B | V | Dist.[′] | Period [days] | Amp. [U/u] | Notes |
|---|---|---|---|---|---|---|---|---|---|
| vEHB-1 | 137.9621546 | −64.87790004 | 18.521 | 19.171 | 19.164 | 1.5 | 3.38683880 | 0.201 | $T_{eff}$ = 20,500 K, No RV variations, HST[49] |
| vEHB-2 | 138.0497832 | −64.86663111 | 18.381 | 18.871 | — | 1.0 | 5.47704961 | 0.181 | HST[49] |
| vEHB-3 | 137.9542449 | −64.83859281 | 19.000 | 19.698 | 19.781 | 2.0 | 26.01823489 | 0.085 | |
| vEHB-4 | 137.9990148 | −64.82868587 | 18.466 | 19.043 | 18.903 | 2.1 | 1.97628738 | 0.074 | |
| vEHB-5 | 137.9939763 | −64.89030570 | 18.955 | 19.565 | 19.337 | 1.7 | 3.23990003 | 0.129 | $T_{eff}$ = 17,900 K[50], No RV variations[50] |
| vEHB-6 | 137.8985627 | −64.82620402 | 18.857 | 19.476 | 19.538 | 3.6 | 50.10395158 | 0.089 | |
| vEHB-7 | 138.0109231 | −64.87461991 | 17.454 | 18.008 | 17.779 | 0.7 | 3.02583807 | 0.082 | HST[49] |
| vEHB-8 | 137.9761837 | −64.85830270 | 18.075 | 18.623 | 18.661 | 0.9 | 2.89086189 | 0.109 | HST[49] |
| vEHB-9 | 137.9968552 | −64.83232443 | 18.588 | 19.126 | 18.817 | 1.9 | 6.90595098 | 0.081 | |
| vEHB-10 | 138.0230711 | −64.89646162 | 17.888 | 18.666 | 18.728 | 2.0 | 3.58179363 | 0.059 | |
| vEHB-11 | 138.0331348 | −64.85209383 | 18.559 | 19.028 | 18.750 | 0.9 | 3.19599005 | 0.091 | HST[49] |
| vEHB-12 | 137.7036732 | −64.85410887 | 18.340 | 18.833 | 19.007 | 7.8 | 4.26386105 | 0.221 | |
| vEHB-13-candidate | 138.0365184 | −64.851004491 | 18.055 | 18.617 | 18.819 | 1.0 | 0.80305948 | 0.075 | HST[49] |
| vEHB-14-candidate | 137.9571663 | −64.903780587 | 18.647 | 19.177 | 18.926 | 2.8 | 11.37292900 | 0.043 | |
| vEHB-15-candidate | 138.0315200 | −64.830937154 | 18.653 | 19.363 | 19.364 | 2.0 | 2.32221267 | 0.041 | |
| vEHB-1/V16 | 287.776790177 | −59.980062960 | 15.598 | 16.404 | 16.608 | 1.8 | 19.54612162 | 0.079 | HST[51], No RV variations |
| vEHB-2/V15 | 287.797182867 | −59.995938057 | 15.444 | 16.199 | 16.358 | 2.6 | 2.27672174 | 0.037 | No RV variations |
| Padua-1 | 287.489983795 | −60.031265955 | 16.174 | 17.092 | 17.348 | 7.4 | lpv | <0.1 | $T_{eff}$ = 29,800 K, No RV variations |
| Padua-2 | 287.686888358 | −59.951220918 | 16.055 | 16.956 | 17.191 | 2.0 | lpv | <0.1 | |
| Padua-3 | 287.698905364 | −59.982337781 | 16.227 | 16.956 | 16.923 | 0.5 | lpv | <0.1 | |
| Padua-4 | 287.678071371 | −59.963366804 | 16.361 | 17.270 | 17.501 | 1.6 | lpv | <0.1 | |
| Padua-5 | 287.652237292 | −59.887642791 | 16.500 | 17.453 | 17.664 | 6.0 | lpv | <0.1 | |
| Padua-6 | 287.658750464 | −60.011251791 | 15.923 | 16.843 | 17.054 | 2.5 | lpv | <0.1 | |
| Padua-7 | 287.628541757 | −59.930214607 | 16.208 | 17.095 | 17.280 | 4.1 | lpv | <0.1 | No RV variations |
| vEHB-3-candidate | 287.676080625 | −60.018833877 | 15.748 | 16.495 | 16.662 | 2.5 | 1.855326900 | 0.043 | |
| vEHB-4/V17-candidate | 287.766889084 | −59.985405659 | 15.410 | 15.370 | 15.311 | 1.5 | 3.287787277 | 0.031 | No RV variations |
| vEHB-1 | 201.745948987 | −47.490663552 | 16.852 | 17.569 | 17.631 | 2.4 | 11.42978680 | 0.177 | HST[52] |
| vEHB-2/NV-380 | 201.594051157 | −47.514662905 | 16.476 | 17.224 | 17.249 | 4.5 | 7.82858823 | 0.132 | $T_{eff}$ = 28,200 K[53], No RV variations[53],HST[52] |
| vEHB-3/NV-404 | 201.591343236 | −47.434931385 | 16.569 | 17.189 | 17.274 | 4.8 | 5.16509016 | 0.107 | HST[52] |
| vEHB-4 | 201.859030855 | −47.443357761 | 16.953 | 17.621 | 17.671 | 7.1 | 4.45548674 | 0.107 | $T_{eff}$ = 24,494 K[54] |
| vEHB-5 | 201.759893238 | −47.419636276 | 17.275 | 18.068 | 18.104 | 4.4 | 2.14022724 | 0.139 | HST[52] |
| vEHB-6 | 201.743567846 | −47.486164373 | 16.989 | 17.742 | 17.849 | 2.2 | 2.06371151 | 0.099 | HST[52] |
| vEHB-7 | 201.822724024 | −47.463627490 | 16.831 | 17.582 | 17.644 | 5.4 | 1.78352993 | 0.071 | $T_{eff}$ = 23,829 K[54] |

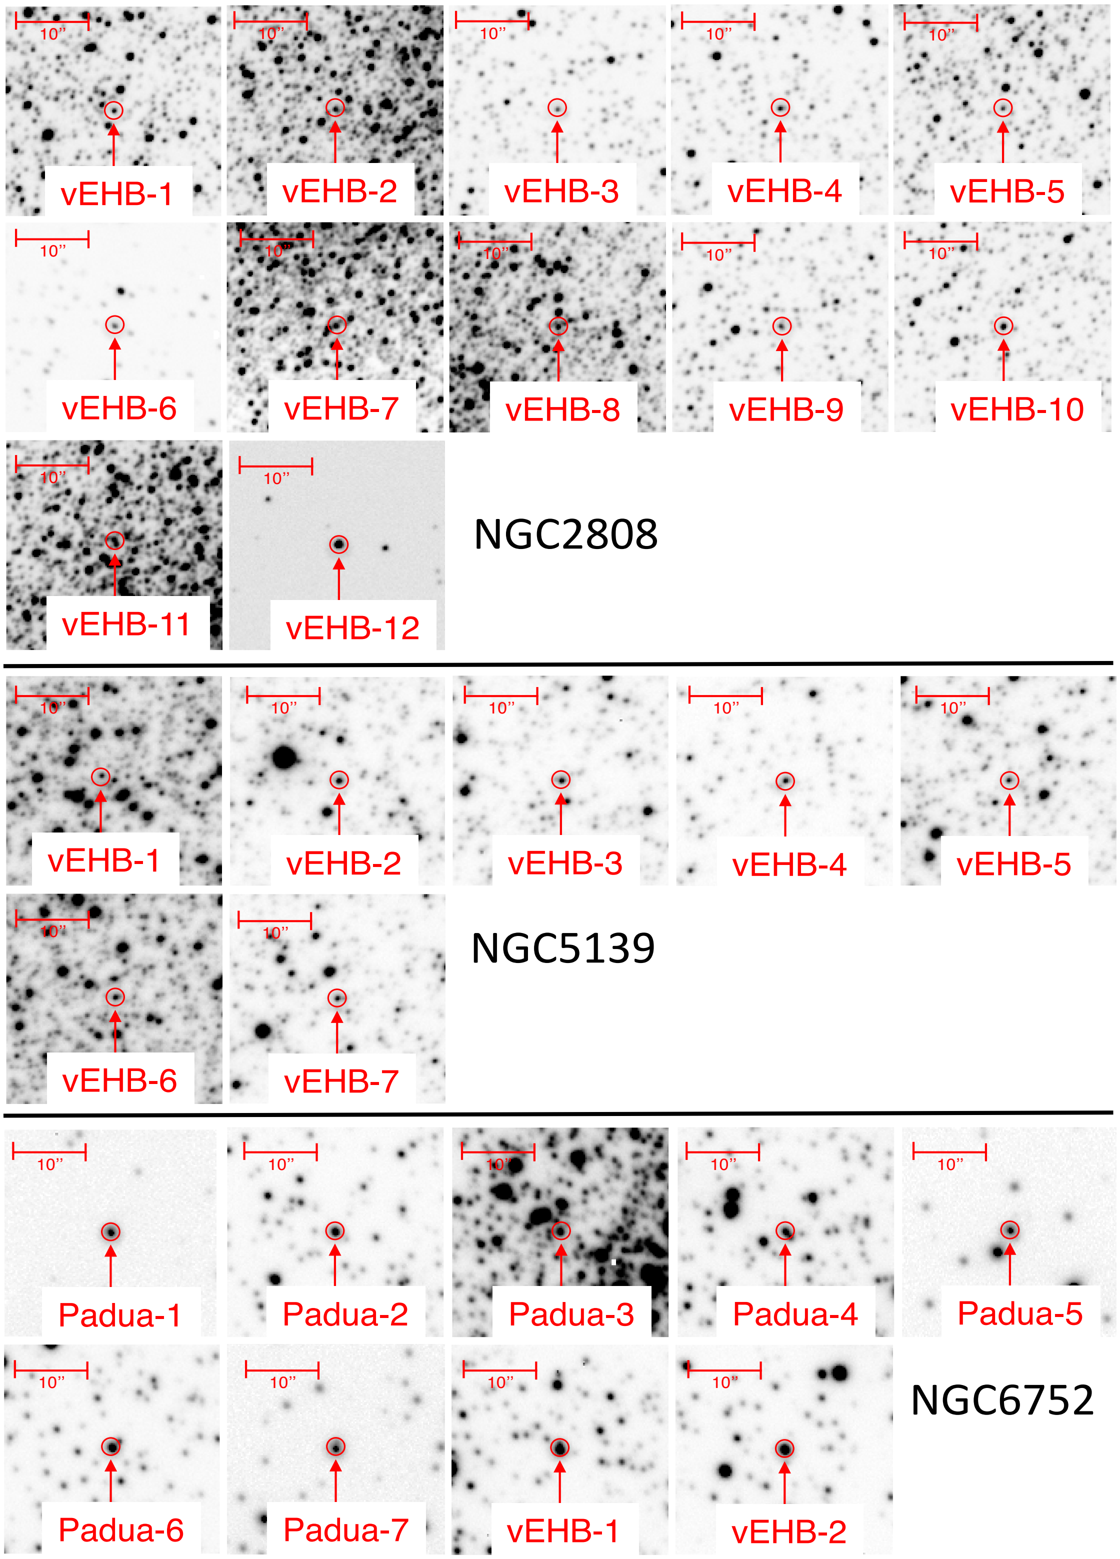


Supplementary Figure 7: Finding charts for our reported EHB and Padua variables. Each chart is 30″ on a side; North is up while East is to the left. The charts are based on our near-ultraviolet Johnson $U_{Johnson}$ filter (NGC2808) and sloan $u_{SDSS}$ filter (NGC6752 and NGC5139) images.
